# Supplementary material for: An Approximate Shading Model with Detail Decomposition for Object Relighting
Source: arXiv:1804.07514 source file (2018-04-20)
Supplement: Supplementary file 1 [file supp.tex]

\clearpage
\begin{center}{\Large Supplemental Material}
\end{center}

\begin{figure}[!th]
\begin{minipage}{0.5\linewidth}
\centering{\large Inset} \\
\includegraphics[width=\linewidth]{cellarvenus_inset.png}\\
\includegraphics[width=\linewidth]{redroom_inset.png}\\
\includegraphics[width=\linewidth]{chapelstone_inset.png}
\end{minipage}
\begin{minipage}{0.5\linewidth}
\centering{\large Insertion result} \\
\includegraphics[width=\linewidth]{cellarvenus_composite_both.png}\\
\includegraphics[width=\linewidth]{redroom_composite_matte.png}\\
\includegraphics[width=\linewidth]{chapelstone_composite.png}
\end{minipage}
\vspace{2mm}
\caption{
Our relighting system adjusts the shading on the object for a variety of scenes with different illumination conditions. Detail composition simulates complex surface geometry and materials properties that is difficult to achieve by physically-based modeling.
}
\vspace{-5mm}
\label{fig:result4}
\end{figure}

\begin{figure}[h]
\begin{minipage}{.495\linewidth}
\centering{\large 3D scene}\\
\includegraphics[width=\linewidth]{muse_orig}\\\vspace{0.5mm}
\includegraphics[width=\linewidth]{tea_orig}
\end{minipage}
\begin{minipage}{.495\linewidth}
\centering{\large Insertion result}\\
\includegraphics[width=\linewidth]{muse_composite_clean}\\\vspace{0.5mm}
\includegraphics[width=\linewidth]{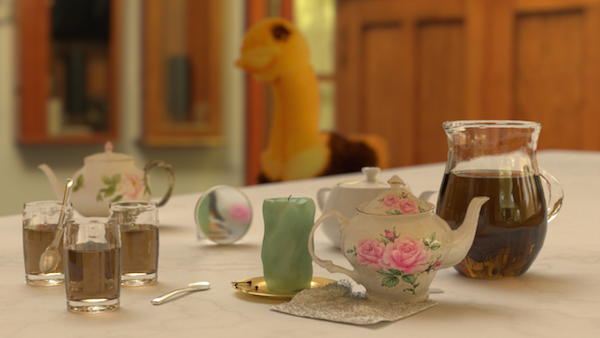}
\end{minipage}
\vspace{2mm}
\caption{Relighting objects into existing 3D graphics scenes. %Pasting the image fragments leads to undesirable results (\emph{middle}). our method allows for objects to live and interact naturally with the rest of the scene (\emph{right}).
Lighting and shadowing of inserted objects appears consistent with the rest of the scene, and our method also captures complex reflection (front teapot), refraction (back teapot) and depth-of-field of effects (ostrich). \emph{Modeling credit to: Jason Clarke (tea scene), ``Carbonflux'' (Sponza scene), and Doug Hammond (HDRI maps)}.}
\label{fig:3Dscenes2}
\end{figure}

%%%%%%%%%%%%%%
\begin{figure}[!th]
\begin{minipage}{0.245\linewidth}
\centering{\large Inset} \\
\includegraphics[width=\linewidth]{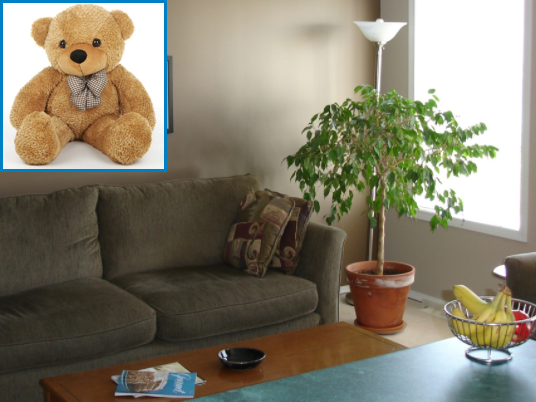}\\\vspace{0.5mm}
\includegraphics[width=\linewidth]{poolroom-kettle_inset_cropped}\\\vspace{0.5mm}
\includegraphics[width=\linewidth]{chairroom-beanbag_inset}\\\vspace{0.5mm}
\includegraphics[width=\linewidth]{table-toy_inset}\\\vspace{0.5mm}
\includegraphics[width=\linewidth]{waterpainting-cube_inset}
\end{minipage}
\begin{minipage}{0.245\linewidth}
\centering{\large Poisson clone} \\
\includegraphics[width=\linewidth]{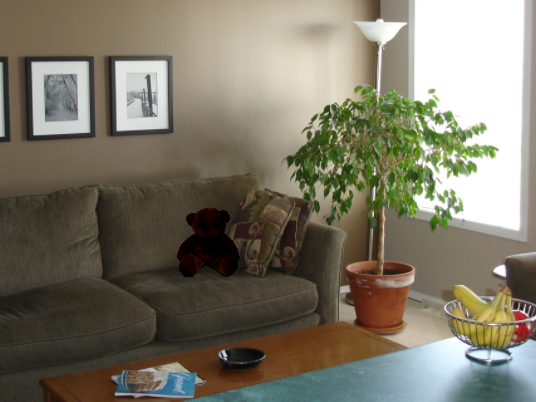}\\\vspace{0.5mm}
\includegraphics[width=\linewidth]{poolroom-kettle_poisson_cropped}\\\vspace{0.5mm}
\includegraphics[width=\linewidth]{chairroom-beanbag_poisson}\\\vspace{0.5mm}
\includegraphics[width=\linewidth]{table-toy_poisson}\\\vspace{0.5mm}
\includegraphics[width=\linewidth]{waterpainting-cube_poisson}
\end{minipage}
\begin{minipage}{0.245\linewidth}
\centering{\large B \& M } \\
\includegraphics[width=\linewidth]{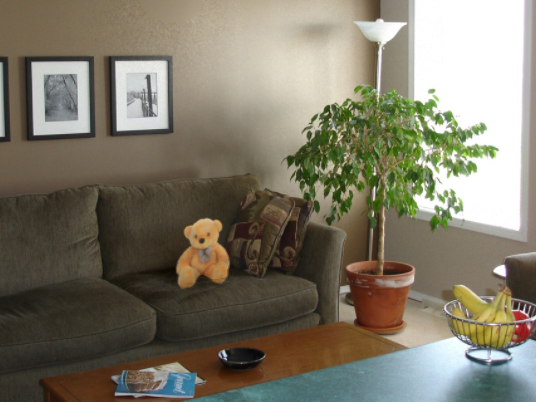}\\\vspace{0.5mm}
\includegraphics[width=\linewidth]{poolroom-kettle_barron_cropped}\\\vspace{0.5mm}
\includegraphics[width=\linewidth]{chairroom-beanbag_barron}\\\vspace{0.5mm}
\includegraphics[width=\linewidth]{table-toy_barron}\\\vspace{0.5mm}
\includegraphics[width=\linewidth]{waterpainting-cube_barron}
\end{minipage}
\begin{minipage}{0.245\linewidth}
\centering{\large Ours} \\
\includegraphics[width=\linewidth]{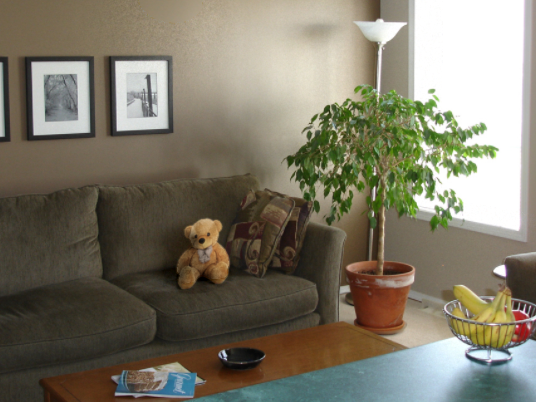}\\\vspace{0.5mm}
\includegraphics[width=\linewidth]{poolroom-kettle_ours_cropped}\\\vspace{0.5mm}
\includegraphics[width=\linewidth]{chairroom-beanbag_ours}\\\vspace{0.5mm}
\includegraphics[width=\linewidth]{table-toy_ours}\\\vspace{0.5mm}
\includegraphics[width=\linewidth]{waterpainting-cube_ours}
\end{minipage}
\vspace{0mm}
\caption{
More relighting results. Column 2 shows results by Poisson cloning~\protect{\cite{Perez:2003:poisson}}.
}
\vspace{-5mm}
\label{fig:result2}
\end{figure}

\clearpage
\begin{figure}[h]
\centering
\begin{tabular}{ccc}
B \& M~\cite{Barron:2012B} & Ours & Real scene\\
\includegraphics[height=.65in]{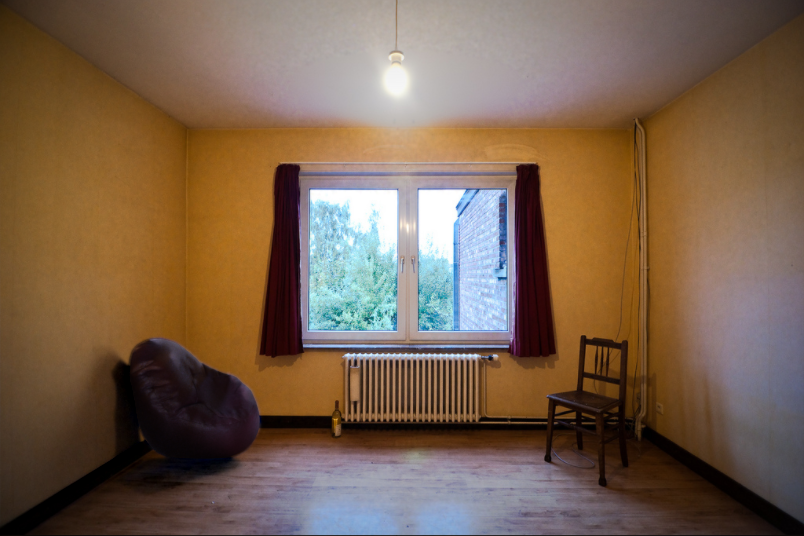}&
\includegraphics[height=.65in]{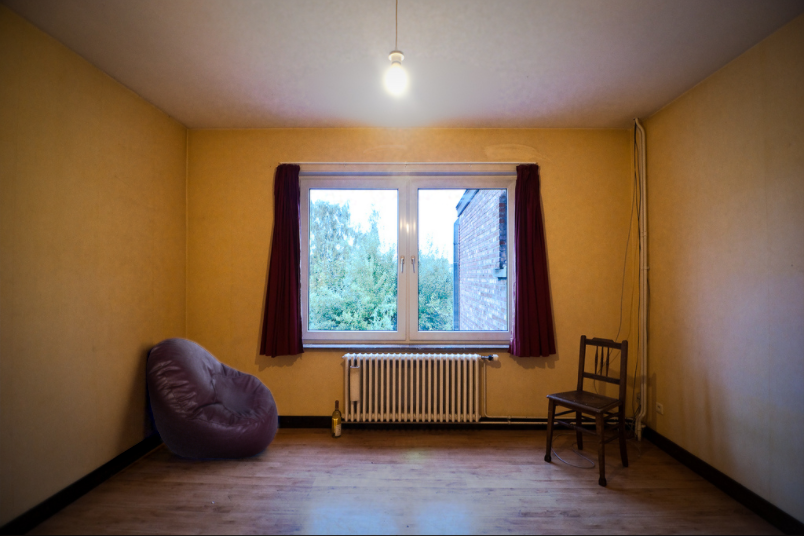}&
\includegraphics[height=.65in]{userstudy_01-r}\\

\includegraphics[height=.65in]{userstudy_02-b}&
\includegraphics[height=.65in]{userstudy_02-o}&
\includegraphics[height=.65in]{userstudy_02-r}\\

\includegraphics[height=.65in]{userstudy_03-b}&
\includegraphics[height=.65in]{userstudy_03-o}&
\includegraphics[height=.65in]{userstudy_03-r}\\

\includegraphics[height=.65in]{userstudy_04-b}&
\includegraphics[height=.65in]{userstudy_04-o}&
\includegraphics[height=.65in]{userstudy_04-r}\\

\includegraphics[height=.65in]{userstudy_05-b}&
\includegraphics[height=.65in]{userstudy_05-o}&
\includegraphics[height=.65in]{userstudy_05-r}\\

\includegraphics[height=.65in]{userstudy_06-b}&
\includegraphics[height=.65in]{userstudy_06-o}&
\includegraphics[height=.65in]{userstudy_06-r}\\

\includegraphics[height=.65in]{userstudy_07-b}&
\includegraphics[height=.65in]{userstudy_07-o}&
\includegraphics[height=.65in]{userstudy_07-r}\\

\includegraphics[height=.65in]{userstudy_08-b}&
\includegraphics[height=.65in]{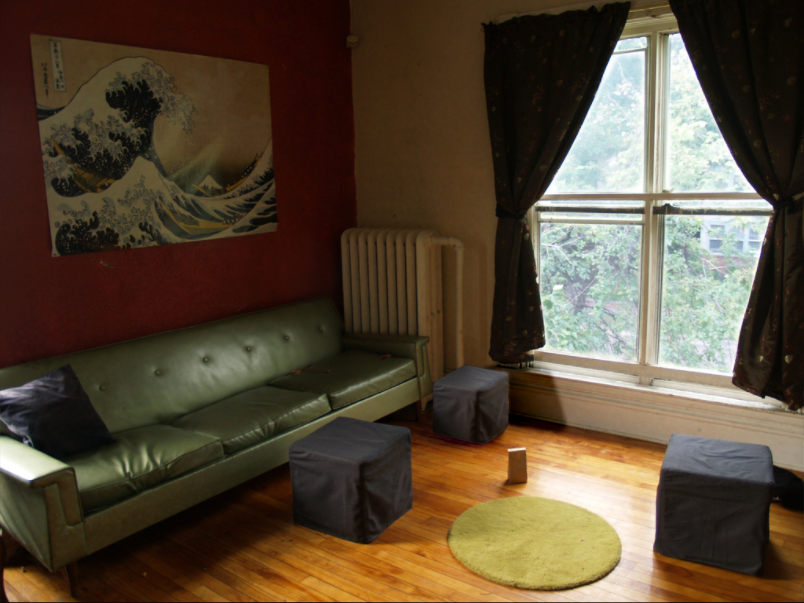}&
\includegraphics[height=.65in]{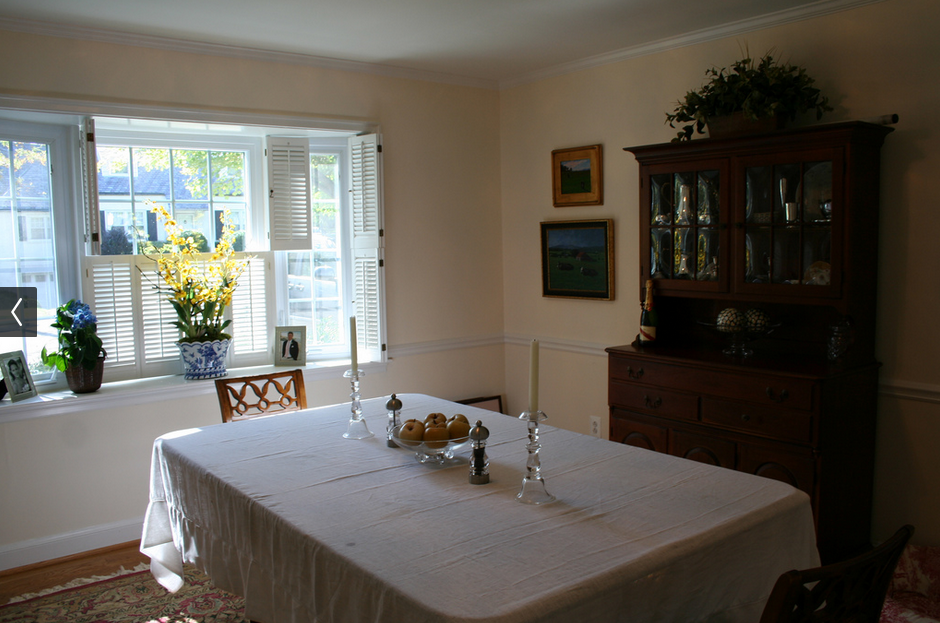}\\

\includegraphics[height=.65in]{userstudy_09-b}&
\includegraphics[height=.65in]{userstudy_09-o}&
\includegraphics[height=.65in]{userstudy_09-r}\\

\includegraphics[height=.65in]{userstudy_10-b}&
\includegraphics[height=.65in]{userstudy_10-o}&
\includegraphics[height=.65in]{userstudy_10-r}
\end{tabular}
\caption{
The 10 image examples in our user study. The first column is the result by Barron and Malik; the second column is by our method; the third column is the real scene corresponding to each insertion example. We would like to make the image set and collected user data publicly available.
}
\vspace{-5mm}
\label{fig:result3}
\end{figure}

%\begin{figure}[h]
%  \centering
%  \includegraphics[width=\textwidth]{../images/failure/head1}\\\vspace{.5mm}%\hfill
%  \includegraphics[width=\textwidth]{../images/failure/head2}
%  \caption{A failure example under extreme lighting conditions. The top row shows a 3D model lit under four lighting conditions: three-quarters direction (3Q), and along each principle axis (left, front, top). The bottom rows shows our results. Our model appears realistic when the lighting is not strongly directed from one side (e.g. 3Q; front), but looks unnatural in harsh conditions (left; top) due to our rough shape estimate. However, such illumination conditions are rare in real pictures, and our models suffice in many cases. Furthermore, relighting our fragments is much more efficient than the alternative of modeling complex human appearance (e.g. skin, hair, etc).
%  }
%  \label{fig:failurecase}
%\end{figure}
